# Supplementary material for: Explorative Imitation Learning: A Path Signature Approach for Continuous Environments
Source: arXiv:2407.04856 source file (2024-07-22)
Supplement: Supplementary file 1 [file dictionary.tex]

% !TeX root = ../../../appendix.tex
% File-name: dictionary.tex
\documentclass{standalone}
\usepackage{tikz}
\usepackage{amsmath}
\usepackage{fix-cm}
\usepackage{graphicx}
\usepackage{mystyle}

\usetikzlibrary{
    matrix,
    decorations, 
    decorations.pathreplacing
}

\begin{document}
\begin{tikzpicture}[]

    % Define matrix
    % \matrix (m) [
    %     matrix of nodes,
    %     nodes in empty cells,
    %     row sep=0pt,
    %     column sep=0pt,
    %     nodes={minimum width=20pt, minimum height=20pt}
    % ]{
    %     1 & & & & & & & & \\
    %     $\beta(\tau)^1_{1, n}$ & $\beta(\tau)^2_{1, n}$ & $\cdots$ & $\beta(\tau)^d_{1, n}$ & & & & & \\
    %     $\beta(\tau)^{1, 1}_{1, n}$ & $\beta(\tau)^{1, 2}_{1, n}$ & $\cdots$ & $\beta(\tau)^{1, d}_{1, n}$ & $\beta(\tau)^{2, 1}_{1, n}$ & $\cdots$ & $\beta(\tau)^{d, 1}_{1, n}$ & $\beta(\tau)^{d, 2}_{1, n}$ & $\cdots$ & $\beta(\tau)^{d, d}_{1, n}$ \\
    %     $\beta(\tau)^{1, 1, 1}_{1, n}$ & $\beta(\tau)^{1, 1, 2}_{1, n}$ & $\cdots$ & $\beta(\tau)^{1, 1, d}$ & $\cdots$ & $\beta(\tau)^{d, d, 1}_{1, n}$ & $\beta(\tau)^{d, d, 2}_{1, n}$ & $\cdots$ & $\beta(\tau)^{d, d, d}$ \\
    %     $\cdots$ \\
    %     $\beta(\tau)^{1, 1, \cdots, 1}_{1, n}$ & & $\cdots$ & $\beta(\tau)^{i_1, i_2, \cdots, i_k}_{1, n}$ & $\cdots$ & $\beta(\tau)^{d, d, \cdots, 1}_{1, n}$ & $\beta(\tau)^{d, d, \cdots, 2}_{1, n}$ & $\cdots$ & $\beta(\tau)^{d, d, \cdots, d}_{1, n}$\\
    % };
    
    \matrix (m) [
        matrix of nodes,
        nodes in empty cells,
        row sep=0pt,
        column sep=3pt,
        nodes={minimum width=20pt, minimum height=20pt}
    ]{
        1 & $\beta(\tau)^1_{1, n}$ & $\beta(\tau)^{1, 1}_{1, n}$ & $\beta(\tau)^{1, 1, 1}_{1, n}$ & $\cdots$ & $\beta(\tau)^{1, 1, \cdots, 1}_{1, n}$ \\
          & $\beta(\tau)^2_{1, n}$ & $\beta(\tau)^{1, 2}_{1, n}$ & $\beta(\tau)^{1, 1, 2}_{1, n}$ & $\cdots$ & $\beta(\tau)^{1, 1, \cdots, 2}_{1, n}$ \\
          & $\vdots$               & $\vdots$                    & $\vdots$                       &          & $\vdots$ \\
          & $\beta(\tau)^d_{1, n}$ & $\beta(\tau)^{1, d}_{1, n}$ & $\beta(\tau)^{1, 1, d}_{1, n}$ & $\cdots$ & $\beta(\tau)^{1, 1 \cdots, d}_{1, n}$ \\
          &                        & $\beta(\tau)^{2, 1}_{1, n}$ & $\beta(\tau)^{1, 2, 1}_{1, n}$ & $\cdots$ & $\beta(\tau)^{i_1, i_2, \cdots, i_k}_{1, n}$ \\
          &                        & $\vdots$                    & $\vdots$                       &          & $\vdots$ \\
          &                        & $\beta(\tau)^{d, 1}_{1, n}$ & $\beta(\tau)^{d, d, 1}_{1, n}$ & $\cdots$ & $\beta(\tau)^{d, d, \cdots, 1}_{1, n}$ \\
          &                        & $\beta(\tau)^{d, 2}_{1, n}$ & $\beta(\tau)^{d, d, 2}_{1, n}$ & $\cdots$ & $\beta(\tau)^{d, d, \cdots, 2}_{1, n}$ \\
          &                        & $\vdots$                    & $\vdots$                       &          & $\vdots$ \\
          &                        & $\beta(\tau)^{d, d}_{1, n}$ & $\beta(\tau)^{d, d, d}_{1, n}$ & $\cdots$ & $\beta(\tau)^{d, d, \cdots, d}_{1, n}$ \\
    };
    
    % Add braces
    \draw [->, >=latex]
        ([xshift=-8pt, yshift=2pt]m-1-1.north west) -- 
        ([yshift=2pt]m-1-6.north east) {};
    %\node [above=2pt] at ([xshift=-13pt]m-1-1.north) {\scriptsize $i$};
    \node [above=2pt] at (m-1-1.north)  {\scriptsize $0$};
    \node [above=2pt] at (m-1-2.north)  {\scriptsize $1$};
    \node [above=2pt] at (m-1-3.north)  {\scriptsize $2$};
    \node [above=2pt] at (m-1-4.north)  {\scriptsize $3$};
    \node [above=2pt] at (m-1-5.north)  {\scriptsize $\cdots$};
    \node [above=2pt] at (m-1-6.north)  {\scriptsize $k$};

    \draw [->, >=latex]
        ([yshift=10pt]m-1-1.north west) --
        (m-10-1.south west) node[midway, left=2pt] {\rotatebox{90}{$d^i\text{ items}$}};
    \node [xshift=-6pt, above=2pt] at (m-1-1.north west) {\scriptsize $i$};
    \node [xshift=10pt, above=12pt] at (m-1-4.north west) {\scriptsize depth};
\end{tikzpicture}
\end{document}
