# Supplementary material for: Explorative Imitation Learning: A Path Signature Approach for Continuous Environments
Source: arXiv:2407.04856 source file (2024-07-22)
Supplement: Supplementary file 2 [file signatures_double.tex]

% !TeX root = ../../../appendix.tex
% File-name: signatures_double.tex
\documentclass{standalone}
\usepackage{tikz}
\usepackage{amsmath}
\usepackage{fix-cm}
\usepackage{mystyle}

\usetikzlibrary{
    matrix,
    decorations, 
    decorations.pathreplacing
}

\begin{document}
\begin{tikzpicture}[]

    % Define matrix
    \matrix (m) [
        matrix of nodes,
        nodes in empty cells,
        row sep=0pt,
        column sep=0pt,
        nodes={minimum width=20pt, minimum height=20pt}
    ]{
        $s^1_1$ & $s^2_1$ & $\cdots$ & $s^d_1$ \\
        $s^1_2$ & $s^2_2$ & $\cdots$ & $s^d_2$ \\
        $\vdots$ & $\vdots$ & $\vdots$ & $\vdots$ \\
        $s^1_n$ & $s^2_n$ & $\cdots$ & $s^d_n$ \\
    };

    % Add braces
    \draw[xshift=-4pt, yshift=0pt] 
        ([xshift=5pt]m-1-4.north) --
        (m-1-4.north east) --
        (m-4-4.south east) --
        ([xshift=5pt]m-4-4.south) {};
    \node [above=1pt] at (m-1-1.north)  {\scriptsize $1$};
    \node [above=1pt] at (m-1-4.north)  {\scriptsize $d$};
    \node [above=1pt] at (m-1-2.north east)  {\scriptsize $\cdots$};

    \draw[xshift=0pt, yshift=-4pt] 
        ([xshift=-5pt]m-1-1.north) --
        (m-1-1.north west) -- 
        (m-4-1.south west) --
        ([xshift=-5pt]m-4-1.south) {};
    \node [left=1pt] at (m-1-1.west)  {\scriptsize $1$};
    \node [left=1pt] at (m-4-1.west)  {\scriptsize $n$};
    \node [left=1pt] at (m-2-1.south west) {\scriptsize $\vdots$};

    \draw [draw=cb_blue]
        ([xshift=-2.5pt, yshift=-3pt]m-1-1.north) -- 
        ([xshift= 3.5pt, yshift=-3pt]m-1-1.north west) -- 
        ([xshift= 3.5pt, yshift= 3pt]m-4-1.south west) --
        ([xshift=-2.5pt, yshift= 3pt]m-4-1.south){};

    \draw [draw=cb_blue]
        ([xshift= 2.5pt, yshift=-3pt]m-1-1.north) -- 
        ([xshift=-3.5pt, yshift=-3pt]m-1-1.north east) -- 
        ([xshift=-3.5pt, yshift= 3pt]m-4-1.south east) --
        ([xshift= 2.5pt, yshift= 3pt]m-4-1.south){};
        
    \draw [draw=cb_blue]
        ([xshift=-2.5pt, yshift=-2pt]m-1-2.north) -- 
        ([xshift=2.5pt, yshift=-2pt]m-1-2.north west) -- 
        ([xshift=2.5pt, yshift=2pt]m-4-2.south west) --
        ([xshift=-2.5pt, yshift=2pt]m-4-2.south){};

    \draw [draw=cb_blue]
        ([xshift=2.6pt, yshift=-2pt]m-1-2.north) -- 
        ([xshift=-2.5pt, yshift=-2pt]m-1-2.north east) -- 
        ([xshift=-2.5pt, yshift=2pt]m-4-2.south east) --
        ([xshift=2.5pt, yshift=2pt]m-4-2.south){};
    \node [below=1pt, text=cb_blue] at (m-4-1.south) {\fontsize{4}{4}\selectfont $\beta(\tau)^{2, 1}_{1, n}$};
    
    \draw [draw=cb_orange]
        ([xshift=-2.5pt, yshift=-3pt]m-1-2.north) -- 
        ([xshift=3.5pt, yshift=-3pt]m-1-2.north west) -- 
        ([xshift=3.5pt, yshift=3pt]m-4-2.south west) --
        ([xshift=-2.5pt, yshift=3pt]m-4-2.south){};

    \draw [draw=cb_orange]
        ([xshift=2.6pt, yshift=-3pt]m-1-2.north) -- 
        ([xshift=-3.5pt, yshift=-3pt]m-1-2.north east) -- 
        ([xshift=-3.5pt, yshift=3pt]m-4-2.south east) --
        ([xshift=2.5pt, yshift=3pt]m-4-2.south){};
    \node [below=1pt, text=cb_orange] at (m-4-2.south) {\fontsize{4}{4}\selectfont $\beta(\tau)^{2, 2}_{1, n}$};
        
    \draw [draw=cb_green]
        ([xshift=-2.5pt, yshift=-1pt]m-1-2.north) -- 
        ([xshift= 1.5pt, yshift=-1pt]m-1-2.north west) -- 
        ([xshift= 1.5pt, yshift= 1pt]m-4-2.south west) --
        ([xshift=-2.5pt, yshift= 1pt]m-4-2.south){};
        
    \draw [draw=cb_green]
        ([xshift=-2.5pt, yshift=-3pt]m-1-4.north) -- 
        ([xshift=3.5pt, yshift=-3pt]m-1-4.north west) -- 
        ([xshift=3.5pt, yshift=3pt]m-4-4.south west) --
        ([xshift=-2.5pt, yshift=3pt]m-4-4.south){};

    \draw [draw=cb_green]
        ([xshift= 2.6pt, yshift=-1pt]m-1-2.north) -- 
        ([xshift=-1.5pt, yshift=-1pt]m-1-2.north east) -- 
        ([xshift=-1.5pt, yshift= 1pt]m-4-2.south east) --
        ([xshift= 2.5pt, yshift= 1pt]m-4-2.south){};

    \draw [draw=cb_green]
        ([xshift=2.6pt, yshift=-3pt]m-1-4.north) -- 
        ([xshift=-3.5pt, yshift=-3pt]m-1-4.north east) -- 
        ([xshift=-3.5pt, yshift=3pt]m-4-4.south east) --
        ([xshift=2.5pt, yshift=3pt]m-4-4.south){};
    \node [below=1pt, text=cb_green] at (m-4-4.south) {\fontsize{4}{4}\selectfont $\beta(\tau)^{2, d}_{1, n}$};
\end{tikzpicture}
\end{document}
