# Supplementary material for: Explorative Imitation Learning: A Path Signature Approach for Continuous Environments
Source: arXiv:2407.04856 source file (2024-07-22)
Supplement: Supplementary file 4 [file stepbystep.tex]

\documentclass{standalone}
\usepackage{tikz}
\usepackage{amsmath,amssymb,amsfonts,amsthm}
\usetikzlibrary{positioning, calc, intersections}

\begin{document}

\begin{tikzpicture}[scale=1.5, node distance=2mm, every node/.style={align=center, anchor=west}]
    % Equation 4
    \node[align=center] (k3) {
        $\begin{aligned}
            \beta(\tau)^{1, 1, 1}_{1, 10} &= \int\!\!\!\!\int\!\!\!\!\int_{1 < t_1 \leqslant t_2 \leqslant t_3 \leqslant 10} d\tau^1_{t_1}d\tau^1_{t_2}d\tau^1_{t_3} = \int_1^{t_1} \left[ \int_1^{t_2} \left[ \int_1^{t_3} dt_1 \right] dt_2 \right] dt_3 = 121.5 \\
            &\vdots
        \end{aligned}$
    };

    % Equation 3
    \node[align=center, above=of k3] (k2) {
        $\begin{aligned}
            \beta(\tau)^{1, 1}_{1, 10} &= \int\!\!\!\!\int_{1 < t_1 \leqslant t_2 \leqslant 10} d\tau^1_{t_1}, d\tau^1_{t_2} = \int_1^{10} \left[ \int_1^{t_2} dt_1 \right] dt_2 = 40.5 \\
            \beta(\tau)^{1, 2}_{1, 10} &= \int\!\!\!\!\int_{1 < t_1 \leqslant t_2 \leqslant 10} d\tau^1_{t_1}, d\tau^2_{t_2} = \int_1^{10} \left[ \int_1^{t_2} dt_1 \right] 2(5 + t_2)dt_2 = 970.5 \\
            \beta(\tau)^{2, 1}_{1, 10} &= \int\!\!\!\!\int_{1 < t_1 \leqslant t_2 \leqslant 10} d\tau^2_{t_1}, d\tau^1_{t_2} = \int_1^{10} \left[ \int_1^{t_2} 2(5+t)dt_1 \right] dt_2 = 730.5 \\
            \beta(\tau)^{2, 2}_{1, 10} &= \int\!\!\!\!\int_{1 < t_1 \leqslant t_2 \leqslant 10} d\tau^2_{t_1}, d\tau^2_{t_2} = \int_1^{10} \left[ \int_1^{t_2} 2(5+t)dt_1 \right] 2(5+t)dt_1 = 17,860.5
        \end{aligned}$
    };
    
    % Equation 2
    \node[above=of k2.north west, anchor=south west] (k1) {
        $\begin{aligned}
            \beta(\tau)^1_{1, 10} &= \int_{1 < t \leqslant 10} dt = \tau^1_{10} - \tau^1_1 = 9\\
            \beta(\tau)^1_{1, 10} &= \int_{1 < t \leqslant 10} dt = \tau^2_{10} - \tau^2_1 = 189
        \end{aligned}$
    };
    
    % Equation 1
    \node[above=of k1.north west, anchor=south west] (k0) {$\beta(\tau)^{\o}_{1, n} = 1$};

    \draw[-, >=latex] ([yshift=-2pt]$(current bounding box.west |- k0.south west)$) -- ([yshift=-2pt]$(current bounding box.east |- k0.south east)$);
    \draw[-, >=latex] ([yshift=-2pt]$(current bounding box.west |- k1.south west)$) -- ([yshift=-2pt]$(current bounding box.east |- k1.south east)$);
    \draw[-, >=latex] ([yshift=-2pt]$(current bounding box.west |- k2.south west)$) -- ([yshift=-2pt]$(current bounding box.east |- k2.south east)$);

    \node[anchor=east] at ([xshift=-2pt]k0.west) {\rotatebox{90}{\scriptsize $k = 0$}};
    \node[anchor=east] at ([xshift=-2pt]k1.west) {\rotatebox{90}{\scriptsize $k = 1$ -- Eq. 3}};
    \node[anchor=east] at ([xshift=-2pt]k2.west) {\rotatebox{90}{\scriptsize $k = 2$ -- Eq. 4}};
    \node[anchor=east] at ([xshift=-2pt]k3.west) {\rotatebox{90}{\scriptsize $k \geqslant 3$ -- Eq. 5}};

\end{tikzpicture}

\end{document}
